# Supplementary material for: Yukawa-Lorentz Symmetry in Non-Hermitian Dirac Materials
Source: arXiv:2308.16907 ancillary file (2024-05-28)
Supplement: Supplementary file 1 [file SM-NH-DSM.pdf]

# Supplemental Material: Yukawa-Lorentz Symmetry in Non-Hermitian Dirac Materials

Vladimir Juričić<sup>1,2</sup> and Bitan Roy<sup>3</sup>

<sup>1</sup>*Departamento de Física, Universidad Técnica Federico Santa María, Casilla 110, Valparaíso, Chile*

<sup>2</sup>*Nordita, KTH Royal Institute of Technology and Stockholm University,  
Hannes Alfvéns väg 12, 106 91 Stockholm, Sweden*

<sup>3</sup>*Department of Physics, Lehigh University, Bethlehem, Pennsylvania, 18015, USA*

The Supplemental Material contains (1) the symmetry analysis of the non-Hermitian Dirac operator in  $d = 2$  and  $d = 3$  [Sec. S1], (2) the details of the calculation of the zero-temperature optical conductivity in  $d = 2$  and  $d = 3$  [Sec. S2], (3) the details of the calculation of the mean-field susceptibilities for different classes of mass orders [Sec. S3], (4) the derivation of the renormalization-group flow equations of the fermionic and bosonic velocities [Sec. S4], (5) some keys details of non-Hermitian Hubbard model in graphene [Sec. S5], (6) the details of the leading order  $\varepsilon$  expansion of the quantum-critical Gross-Neveu-Yukawa theory [Sec. S6].

## S1. SYMMETRY ANALYSIS OF THE NON-HERMITIAN DIRAC OPERATOR

We here present the details of the symmetry analysis of the non-Hermitian (NH) Dirac operator, appearing in Eq. (2) of the main text, which can be explicitly rewritten as

$$H_{\text{NH}} = (v_{\text{H}} + v_{\text{NH}} M) \sum_{j=1}^d \Gamma_j k_j \equiv h_0 + h_1, \quad (\text{S1})$$

where  $v_{\text{H}}$  and  $v_{\text{NH}}$  are real parameters, defined in the main text, and the four-component Hermitian matrices  $\Gamma_j$  for  $j = 1, \dots, d$  and the mass matrix  $M$  mutually anticommute. All of them square to the identity matrix. Below we discuss the symmetry protection of the NH Dirac nodes in  $d = 2$  and  $d = 3$  separately in two subsequent subsections.

### A. Two dimensions ( $d = 2$ )

In  $d = 2$ , without any loss of generality, we can choose two kinetic energy matrices  $\Gamma_1$  and  $\Gamma_2$  appearing in the definition of  $h_0$  to be purely imaginary. The mass matrix  $M \in \{M_1, M_2, M_3, \Gamma_{12}\}$ , where  $\Gamma_{jk} = i\Gamma_j\Gamma_k$  in  $d = 2$ , such that  $\{M, h_0\} = 0$ . Then,  $M_1$ ,  $M_2$  and  $M_3$  are purely real, while  $\Gamma_{12}$  is purely imaginary by construction. Therefore,  $\{\Gamma_1, \Gamma_2, M_1, M_2, M_3\}$  constitute the set of five mutually anticommuting Hermitian four-component matrices, each of which squares to the identity matrix.

In Table I of the main text, we show the symmetry transformation of all the possible mass terms of this operator ( $H_{\text{NH}}$ ) in  $d = 2$  for a specific choice of  $M = M_1$  (real). It shows that we cannot add any constant mass term to this NH Dirac operator without breaking any one of the four discrete nonspatial symmetries, namely, time-reversal, unitary and anti-unitary particle-hole symmetries, and pseudo-Hermiticity. The same conclusion can immediately be arrived at for  $M = M_2$  and  $M_3$  due to the reality condition of these two Hermitian mass matrices.

It turns out that when we choose the matrix  $M$  to be purely imaginary, namely  $M = \Gamma_{12}$ , the NH Dirac operator in Eq. (S1) breaks the time-reversal symmetry, generated by  $\mathcal{T}_+ = T_+ \mathcal{K}$ , where  $T_+$  is a unitary operator and  $\mathcal{K}$  is the complex conjugation. Namely, the invariance of the NH Dirac operator in Eq. (S1) with  $M = \Gamma_{12}$  under  $\mathcal{T}_+$ , implies that  $[T_+, \Gamma_i] = 0$ , for  $i = 1, 2$ , and  $\{T_+, \Gamma_{12}\} = 0$ . However, these two conditions are obviously incompatible. Similarly, such a NH Dirac operator cannot feature antiunitary  $\mathcal{T}_-$  and  $\mathcal{C}_+$  symmetries, and unitary pseudo-Hermiticity (PSH). The transformation of the four mass terms under the remaining symmetries, namely the antiunitary particle-hole ( $\mathcal{C}_-$ ) and the unitary particle-hole (PH), is given in Table S1. Therefore, neither of these constant four mass terms can be added to the NH Dirac operator  $H_{\text{NH}}$  with  $M = \Gamma_{12}$  without breaking at least one of the remaining two nonspatial symmetries. Therefore, the form of the NH Dirac operator in  $d = 2$ , given by Eq. (S1), is always protected by the discrete nonspatial symmetries.

| Mass terms    | Symmetries        |                   |                   |                           |       |       |       |               |
|---------------|-------------------|-------------------|-------------------|---------------------------|-------|-------|-------|---------------|
|               | $\mathcal{C}_-$   |                   |                   |                           | PH    |       |       |               |
|               | $M_1 \mathcal{K}$ | $M_2 \mathcal{K}$ | $M_3 \mathcal{K}$ | $\Gamma_{12} \mathcal{K}$ | $M_1$ | $M_2$ | $M_3$ | $\Gamma_{12}$ |
| $M_1$         | ×                 | ✓                 | ✓                 | ×                         | ×     | ✓     | ✓     | ×             |
| $M_2$         | ✓                 | ×                 | ✓                 | ×                         | ✓     | ×     | ✓     | ×             |
| $M_3$         | ✓                 | ✓                 | ×                 | ×                         | ✓     | ✓     | ×     | ×             |
| $\Gamma_{12}$ | ✓                 | ✓                 | ✓                 | ✓                         | ×     | ×     | ×     | ×             |

Table S1. Nonspatial symmetries of the NH Dirac operator in  $d = 2$ ,  $H_{\text{NH}} = (v_{\text{H}} + v_{\text{NH}} M)(\Gamma_1 k_x + \Gamma_2 k_y)$ , with  $M = \Gamma_{12} = i\Gamma_1 \Gamma_2$  [see also Eq. (S1)]. Notice that only two such symmetries are allowed in this case:  $\mathcal{C}_-$  (PH) representing antiunitary (unitary) particle-hole symmetry, acting as  $\mathcal{C}_- H_{\text{NH}}^\dagger \mathcal{C}_-^{-1} = -H_{\text{NH}}$  ( $\text{PH} H_{\text{NH}} \text{PH}^{-1} = -H_{\text{NH}}$ ). We work with a representation in which Hermitian matrices  $M_1$ ,  $M_2$  and  $M_3$  ( $\Gamma_1$  and  $\Gamma_2$ ) are purely real (imaginary). The symbol ✓ (×) indicates whether a mass term is even (odd) under a specific symmetry. Notice that none of the four possible uniform mass terms is invariant under both the nonspatial symmetries of  $H_{\text{NH}}$ , and thus cannot be added to  $H_{\text{NH}}$  without breaking at least one of these symmetries.

### B. Three dimensions ( $d = 3$ )

In  $d = 3$ , the time-reversal symmetry enforces the Hermitian matrices  $\Gamma_i$  with  $i = 1, 2, 3$  in the Hermitian kinetic term ( $h_0$ ) to be purely real. So the remaining two Hermitian matrices  $M_1$  and  $M_2$  in the set of five mutually anticommuting ones are purely imaginary. This set is now explicitly given by  $\{\Gamma_1, \Gamma_2, \Gamma_3, M_1, M_2\}$ . Therefore, the matrix  $M$  in the NH Dirac operator must be purely imaginary and we take it to be  $M = M_1$  for the sake of concreteness. Such an NH Dirac operator enjoys all four discrete nonspatial symmetries, with the corresponding representations shown in Table S2. It shows that neither of the two possible uniform mass terms,  $M_1$  and  $M_2$ , can be added to this NH Dirac operator without breaking one of these discrete symmetries. Therefore, the form of the NH Dirac operator in Eq. (S1) is symmetry protected in  $d = 3$  as well.

## S2. OPTICAL CONDUCTIVITY

In this section, we show the details of the calculation of the zero-temperature optical conductivity in  $d = 2$  and  $d = 3$ , leading to Eq. (4) in the main text. The polarization tensor, with the corresponding diagram displayed in Fig. S1(a), explicitly reads as

$$\Pi_{jj}(i\omega) = -\text{Tr} \int_{-\infty}^{\infty} \frac{d\nu}{2\pi} \int \frac{d^d \mathbf{k}}{(2\pi)^d} [J_j G_{\text{F}}(i\omega + i\nu, \mathbf{k}) J_j G_{\text{F}}(i\nu, \mathbf{k})], \quad (\text{S2})$$

where  $j = 1, \dots, d$ , and the current operator  $J_j = (v_{\text{H}} + v_{\text{NH}} M)\Gamma_j$ , and

$$G_{\text{F}}(i\omega, \mathbf{k}) = \frac{i\omega + H_{\text{NH}}}{\omega^2 + v_{\text{F}}^2 k^2} \quad (\text{S3})$$

is the fermionic Green's function corresponding to the NH Dirac operator in Eq. (S1) with  $v_{\text{F}}^2 = v_{\text{H}}^2 - v_{\text{NH}}^2$ . The rotational symmetry implies isotropy of the polarization tensor. After subtracting its zero-frequency part, the diagonal element of the polarization tensor  $\Pi(i\omega) = (1/d) \sum_{j=1}^d [\Pi_{jj}(i\omega) - \Pi_{jj}(0)]$ , explicitly reads as

$$\Pi(i\omega) = \frac{4N_f}{d v_{\text{F}}^{d-2}} \int_{-\infty}^{\infty} \frac{d\nu}{2\pi} \int \frac{d^d \mathbf{k}}{(2\pi)^d} \left[ \frac{\nu(\nu + \omega)}{((\omega + \nu)^2 + k^2)(\nu^2 + k^2)} - \frac{\nu^2}{(\nu^2 + k^2)^2} \right], \quad (\text{S4})$$

and we rescaled  $v_{\text{F}} k \rightarrow k$ .

We now set  $d = 2$  in Eq. (S4), and after performing a straightforward algebra, we obtain

$$\Pi(i\omega) = -N_f \frac{\omega}{8}. \quad (\text{S5})$$

| Mass terms | Symmetries        |                   |                   |                           |       |       |
|------------|-------------------|-------------------|-------------------|---------------------------|-------|-------|
|            | $\mathcal{T}_+$   | $\mathcal{C}_+$   | $\mathcal{T}_-$   | $\mathcal{C}_-$           | PH    | PSH   |
|            | $M_1 \mathcal{K}$ | $M_2 \mathcal{K}$ | $M_3 \mathcal{K}$ | $\Gamma_{12} \mathcal{K}$ | $M_1$ | $M_2$ |
| $M_1$      | ✓                 | ×                 | ×                 | ✓                         | ×     | ×     |
| $M_2$      | ×                 | ✓                 | ×                 | ✓                         | ✓     | ×     |

Table S2. Nonspatial symmetries of the NH Dirac operator in  $d = 3$ ,  $H_{\text{NH}} = (v_{\text{H}} + v_{\text{NH}} M)(\Gamma_1 k_x + \Gamma_2 k_y + \Gamma_3 k_z)$ , with  $M = M_1$  [see also Eq. (S1)]. Here,  $\mathcal{T}_+$  and  $\mathcal{C}_+$  ( $\mathcal{T}_-$  and  $\mathcal{C}_-$ ) represent time-reversal (antiunitary particle-hole) symmetry, while PH (PSH) are unitary particle-hole (pseudo-Hermiticity) symmetry, under which  $\mathcal{T}_{\pm} H_{\text{NH}} \mathcal{T}_{\pm}^{-1} = \pm H_{\text{NH}}$ ,  $\mathcal{C}_{\pm} H_{\text{NH}}^{\dagger} \mathcal{C}_{\pm}^{-1} = \pm H_{\text{NH}}$ ,  $\text{PH} H_{\text{NH}} \text{PH}^{-1} = -H_{\text{NH}}$  and  $\text{PSH} H_{\text{NH}}^{\dagger} \text{PSH}^{-1} = H_{\text{NH}}$ . Here we work with a representation of mutually anticommuting four-component Hermitian matrices in which  $\Gamma_1$ ,  $\Gamma_2$  and  $\Gamma_3$  ( $M_1$  and  $M_2$ ) are purely real (imaginary). The notations are identical as in Table S1. Notice that neither of two possible uniform mass terms is invariant under all the discrete nonspatial symmetries of  $H_{\text{NH}}$ , and thus can not be added to  $H_{\text{NH}}$  without breaking at least one of these symmetries.

Finally, the optical conductivity in  $d = 2$  reads as

$$\sigma(\omega) = \frac{\text{Im } \Pi(i\omega \rightarrow \omega + i\eta)}{\omega} \Big|_{\eta \rightarrow 0} = N_f \frac{\pi}{4} \sigma_0, \quad (\text{S6})$$

where  $\sigma_0 = e^2/h$ , with  $e$  as the electron charge and  $h$  as the Planck's constants. This is the result in Eq. (4) of the main text.

In  $d = 3$ , using Eq. (S4), after carrying out straightforward algebra, we find

$$\Pi(i\omega) = -\frac{2N_f \omega^2}{3\pi^2 v_{\text{F}}} \int_0^{\Lambda v_{\text{F}}} \frac{k dk}{k^2 + 4v_{\text{F}}^2}, \quad (\text{S7})$$

with  $\Lambda$  as the ultraviolet momentum cutoff. We then obtain

$$\Pi(i\omega) = -\frac{N_f \omega^2}{12\pi^2 v_{\text{F}}} \ln \left[ 1 + \left( \frac{2\Lambda v_{\text{F}}}{\omega} \right)^2 \right], \quad (\text{S8})$$

yielding the optical conductivity of the NH Dirac fermions in  $d = 3$ ,

$$\sigma(\omega) = \frac{\text{Im } \Pi(i\omega \rightarrow \omega + i\eta)}{\omega} \Big|_{\eta \rightarrow 0} = \frac{N_f \omega}{6v_{\text{F}}} \sigma_0, \quad (\text{S9})$$

which is the result shown in Eq. (4) of the main text.

### S3. MEAN-FIELD SUSCEPTIBILITIES

In this section, we provide the details of the calculation of the mean-field susceptibilities, shown in Eq. (5) of the main text. The susceptibility corresponding to the order-parameter represented by matrix  $N$  at zero external frequency and momentum is

$$\chi_N = -\text{Tr} \int' \frac{d^d \mathbf{k}}{(2\pi)^d} \int \frac{d\omega}{2\pi} [N G_{\text{F}}(i\omega, \mathbf{k}) N G_{\text{F}}(i\omega, \mathbf{k})], \quad (\text{S10})$$

where the fermionic Green's function  $G_{\text{F}}(i\omega, \mathbf{k})$  is given in Eq. (S3), and an upper cutoff ( $\Lambda$ ) is assumed in the momentum integral (denoted by the 'prime' symbol). Here, we consider  $N$  to be a mass matrix, such that  $\{N, h_0\} = 0$ . After performing a straightforward algebra, the susceptibility takes the form

$$\chi_N = 4N_f \int' \frac{d^d \mathbf{k}}{(2\pi)^d} \int \frac{d\omega}{2\pi} \frac{\omega^2 + (v_{\text{H}}^2 \mp v_{\text{NH}}^2)k^2}{(\omega^2 + v_{\text{F}}^2 k^2)^2}, \quad (\text{S11})$$

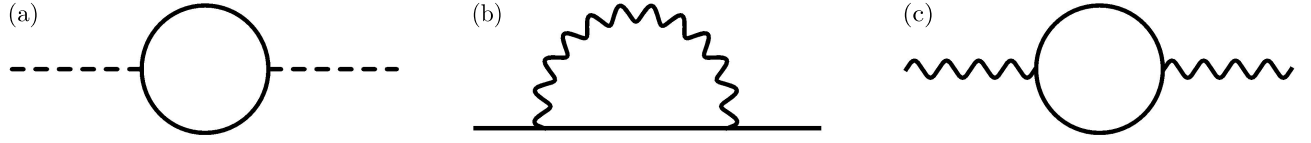

Figure S1. (a) Polarization diagram for the Dirac fermion (solid lines) with dashed lines representing an external electromagnetic field. Self-energy diagrams for the Dirac fermion [(b)] and the bosonic order parameter field (wavy lines) [(c)]. The vertex in (b) and (c) corresponds to the Yukawa coupling in Eq. (S14).

where the upper [lower] sign corresponds to the commuting class mass (CCM), satisfying  $[N, M] = 0$  [anticommuting class mass (ACM), satisfying  $\{N, M\} = 0$ ]. For the CCM, after a straightforward integration, we obtain

$$\chi_N^{(\text{CCM})} = 2N_f \frac{S_d}{(2\pi)^d} \frac{\Lambda^{d-1}}{v_F} \frac{1}{d-1} \equiv N_f f(d) \frac{\Lambda^{d-1}}{v_F}, \quad (\text{S12})$$

with  $f(d) = 2S_d/[(d-1)(2\pi)^d]$  and  $S_d = 2\pi^{d/2}/\Gamma(d/2)$ , while for the ACM case, we find

$$\chi_N^{(\text{ACM})} = \chi_N^{(\text{CCM})} + 2N_f \frac{S_d}{(2\pi)^d} \frac{v_{\text{NH}}^2}{v_F^2} \frac{\Lambda^{d-1}}{v_F} = \chi_N^{(\text{CCM})} \left( 1 + \frac{v_{\text{NH}}^2}{v_F^2} \right), \quad (\text{S13})$$

which is Eq. (5) in the main text, where for notational brevity we used  $\chi_N^{(\text{CCM})} \rightarrow \chi_1$  and  $\chi_N^{(\text{ACM})} \rightarrow \chi_2$ .

#### S4. RENORMALIZATION-GROUP FLOW EQUATIONS OF THE VELOCITIES

In this section, we present the details of the renormalization group (RG) analysis leading to the form of the RG flow equations of the fermionic and bosonic velocities, given by Eqs. (7)-(11) in the main text. To this end, we employ the leading-order  $\varepsilon$  expansion about  $d = 3$  upper critical spatial dimensions of the NH Gross-Neveu-Yukawa (GNY) theory with  $\varepsilon = 3 - d$ . We compute the self-energy diagrams for the fermions and bosons, shown in Figs. S1(b) and (c), respectively, while the Yukawa boson-fermion interaction is given by Eq. (6) in the main text, which explicitly reads

$$S_Y = g \int d\tau \int d^d \mathbf{x} \sum_{j=1}^n \Phi_j(\tau, \mathbf{x}) \Psi^\dagger(\tau, \mathbf{x}) N_j \Psi(\tau, \mathbf{x}), \quad (\text{S14})$$

with  $n$  as the number of the components of the order-parameter and  $\tau$  as the imaginary time.

##### A. Fermionic self-energy

The fermionic self-energy at the external Matsubara frequency  $\nu$  and momentum  $\mathbf{k}$  takes the form

$$\Sigma(i\nu, \mathbf{k}) = g^2 \int \frac{d^d \mathbf{q}}{(2\pi)^d} \int \frac{d\omega}{2\pi} N_i G_F(i\omega, \mathbf{q}) N_i G_B(i(\nu - \omega), \mathbf{k} - \mathbf{q}) \equiv g^2 N_i I(i\nu, \mathbf{k}) N_i, \quad (\text{S15})$$

with the summation over the repeated indices assumed. The fermionic Green's function is given by Eq. (S3), while the bosonic propagator is

$$G_B(i\omega, \mathbf{k}) = \frac{1}{\omega^2 + v_B^2 k^2}. \quad (\text{S16})$$

The divergent piece of the integral  $I(i\nu, \mathbf{k})$  can be found after using the standard Feynman parametrization, yielding

$$I(i\nu, \mathbf{k}) = \frac{1}{4\pi^2 \varepsilon} \frac{1}{v_B (v_F + v_B)^2} \left[ i\nu + \frac{1}{3} (v_H + v_{\text{NH}} M) \Gamma_j k_j \left( 1 + \frac{2v_B}{v_F} \right) \right]. \quad (\text{S17})$$

Finally, the self-energy reads

$$\Sigma^\pm(i\nu, \mathbf{k}) = \frac{g^2}{4\pi^2\varepsilon} \frac{n}{v_B(v_F + v_B)^2} \left[ i\nu - \frac{1}{3}(v_H \pm v_{NH}M)\Gamma_j k_j \left( 1 + \frac{2v_B}{v_F} \right) \right], \quad (\text{S18})$$

where the upper (lower) sign corresponds to the CCM (ACM) order-parameter.

The RG condition

$$Z_\Psi^\pm + \frac{\partial \Sigma^\pm(i\nu, \mathbf{k})}{\partial(i\nu)} \Big|_{i\nu=0, \mathbf{k}=0} = 1, \quad (\text{S19})$$

yields the fermionic field renormalization  $Z_\Psi^\pm$  for the two classes of the order-parameters

$$Z_\Psi \equiv Z_\Psi^\pm = 1 - \frac{g^2}{4\pi^2\varepsilon} \frac{n}{v_B(v_F + v_B)^2}, \quad (\text{S20})$$

which is independent of the order-parameter class. Using Eq. (S18), we find the conditions for the renormalization constants corresponding to the parameters  $v_H$  and  $v_{NH}$  in the CCM class, given by

$$Z_\Psi Z_{v_H}^+ = Z_\Psi Z_{v_{NH}}^+ = 1 - \frac{g^2}{4\pi^2\varepsilon} \frac{n}{v_B(v_F + v_B)^2} \left( 1 + \frac{2v_B}{v_F} \right), \quad (\text{S21})$$

while for the ACM class, we obtain

$$Z_\Psi Z_{v_H}^- = 1 - \frac{g^2}{4\pi^2\varepsilon} \frac{n}{v_B(v_F + v_B)^2} \left( 1 + \frac{2v_B}{v_F} \right), \quad (\text{S22})$$

$$Z_\Psi Z_{v_{NH}}^- = 1 + \frac{g^2}{4\pi^2\varepsilon} \frac{n}{v_B(v_F + v_B)^2} \left( 1 + \frac{2v_B}{v_F} \right). \quad (\text{S23})$$

Therefore, the renormalization constants  $Z_{v_H}^\pm$  and  $Z_{v_{NH}}^\pm$  are given by

$$Z_{v_H}^\pm = Z_{v_{NH}}^+ = 1 + \frac{g^2}{4\pi^2\varepsilon} \frac{n}{v_B(v_F + v_B)^2} \left( \frac{2}{3} \right) \left( 1 - \frac{v_B}{v_F} \right), \quad (\text{S24})$$

$$Z_{v_{NH}}^- = 1 + \frac{g^2}{4\pi^2\varepsilon} \frac{n}{v_B(v_F + v_B)^2} \left( \frac{4}{3} \right) \left( 1 + \frac{v_B}{2v_F} \right). \quad (\text{S25})$$

The renormalization condition for each of the velocities  $Z_{v_\alpha} v_\alpha = v_\alpha^0$ , with  $\alpha = H, NH$ , and  $v_\alpha^0$  as the corresponding bare velocities, implies the form of the  $\beta$ -functions given in Eqs. (7), (8), and (10) of the main text.

## B. Bosonic self-energy

We now turn to the bosonic self-energy to determine the RG flow of the bosonic velocities. The bosonic self-energy, given by the diagram in Fig. S1(c), is

$$\Pi(i\nu, \mathbf{k}) = -\frac{g^2}{2} \int \frac{d^d \mathbf{q}}{(2\pi)^d} \int \frac{d\omega}{2\pi} \text{Tr} [N_i G_F(i\omega, \mathbf{q}) N_i G_F(i\nu + i\omega, \mathbf{k} + \mathbf{q})]. \quad (\text{S26})$$

After some algebra, the bosonic self-energy can be written as

$$\Pi^\pm(i\nu, \mathbf{k}) = 2g^2 n N_f J_\pm(i\nu, \mathbf{k}), \quad (\text{S27})$$

where

$$J_\pm(i\nu, \mathbf{k}) = \int \frac{d^d \mathbf{q}}{(2\pi)^d} \int \frac{d\omega}{2\pi} \frac{\omega(\omega + \nu) + (v_H^2 \mp v_{NH}^2) \mathbf{q} \cdot (\mathbf{k} + \mathbf{q})}{(\omega^2 + v_F^2 q^2)[(\omega + \nu)^2 + v_F^2 (\mathbf{k} + \mathbf{q})^2]}, \quad (\text{S28})$$

with the upper (lower) sign corresponding to the CCM (ACM) order parameter. A straightforward integration then yields

$$J_{\pm}(i\nu, \mathbf{k}) = \frac{\Gamma\left(\frac{3-d}{2}\right) \left[\Gamma\left(\frac{1+d}{2}\right)\right]^2}{4(4\pi)^{d/2} v_F^3 (1-d) \Gamma(3/2) \Gamma(d+1)} \left(k^2 + \frac{\nu^2}{v_F^2}\right)^{\frac{d-3}{2}} \left[d \left(1 + \frac{f_{\pm}^2}{v_F^2}\right) \nu^2 + ((2d-1)f_{\pm}^2 + v_F^2) k^2\right], \quad (\text{S29})$$

where

$$f_{\pm}^2 = v_H^2 \mp v_{\text{NH}}^2. \quad (\text{S30})$$

We then obtain for the bosonic self energy  $\Pi^+(i\nu, \mathbf{k})$  [ $\Pi^-(i\nu, \mathbf{k})$ ] for the CCM (ACM) order parameter, where

$$\Pi^{\pm}(i\nu, \mathbf{k}) = -\frac{g^2 n N_f}{8\pi^2 v_F^3 \epsilon} A_{\pm} (\nu^2 + B_{\pm} v_F^2 k^2), \quad (\text{S31})$$

with

$$A_+ = B_+ = 1, \quad A_- = \left(\frac{v_H}{v_F}\right)^2, \quad B_- = 1 + \frac{2v_{\text{NH}}^2}{3v_H^2}, \quad (\text{S32})$$

which implies that the bosonic field renormalization for the two classes reads

$$Z_{\Phi}^{\pm} = 1 - \frac{g^2 n N_f}{8\pi^2 v_F^3 \epsilon} A_{\pm}, \quad (\text{S33})$$

while the bosonic velocity renormalization factor is given by

$$Z_{\Phi}^{\pm} Z_{v_B^2}^{\pm} = 1 - \frac{g^2 n N_f}{8\pi^2 v_F^3 \epsilon} \left(\frac{v_F^2}{v_B^2}\right) A_{\pm} B_{\pm}. \quad (\text{S34})$$

We therefore find

$$Z_{v_B^2}^+ = 1 + \frac{g^2 n N_f}{8\pi^2 v_F^3 \epsilon} \left(1 - \frac{v_F^2}{v_B^2}\right), \quad (\text{S35})$$

$$Z_{v_B^2}^- = 1 + \frac{g^2 n N_f}{8\pi^2 v_F^3 \epsilon} \left(\frac{v_H^2}{v_F^2} - \frac{v_H^2}{v_B^2} - \frac{2v_{\text{NH}}^2}{3v_B^2}\right), \quad (\text{S36})$$

which after imposing the renormalization conditions  $Z_{v_B^2}^{\pm} (v_B^{\pm})^2 = (v_B^{\pm,0})^2$ , with  $v_B^{\pm,0}$  as the corresponding bare velocities, yields the RG flow equations in Eqs. (9) and (11) of the main text for the fluctuations of the CCM and ACM order parameters, respectively.

## S5. NON-HERMITIAN HUBBARD MODEL IN GRAPHENE

The Dirac quasiparticles arise in graphene from the nearest-neighbor hopping process of free fermions that can be captured in terms of a two component spinor  $\Psi_{\mathbf{k}}^{\top} = (c_A, c_B)(\mathbf{k})$ , where  $c_A(\mathbf{k})$  and  $c_B(\mathbf{k})$  are the fermionic annihilation operators on the sites of two interpenetrating triangular sublattices  $A$  and  $B$ , respectively. In this basis, the tight-binding Hamiltonian with only nearest-neighbor hopping ( $t_0$ ) reads as

$$h_0^{\text{lat}}(\mathbf{k}) = t_0 \begin{pmatrix} 0 & f(\mathbf{k}) \\ f^*(\mathbf{k}) & 0 \end{pmatrix}, \quad (\text{S37})$$

where  $f(\mathbf{k}) = \exp[i\mathbf{k} \cdot \mathbf{b}_1] + \exp[i\mathbf{k} \cdot \mathbf{b}_2] + \exp[i\mathbf{k} \cdot \mathbf{b}_3]$ , and  $\mathbf{b}_1 = (1/\sqrt{3}, 1)a/2$ ,  $\mathbf{b}_2 = (1/\sqrt{3}, -1)a/2$  and  $\mathbf{b}_3 = (-1/\sqrt{3}, 0)a$  are the nearest-neighbor vectors. Here  $a$  is the lattice spacing and ‘ $\star$ ’ denotes the complex conjugation. The inclusion of the spin degrees of freedom leads to a mere doubling of  $h_0^{\text{lat}}(\mathbf{k})$ , and for spinful fermions the tight-binding lattice Hamiltonian takes the form  $\sigma_0 h_0^{\text{lat}}(\mathbf{k})$ , where the two-component Pauli matrices  $\{\sigma_{\mu}\}$  operate on the spin indices, with  $\mu = 0, 1, 2, 3$ . In this language, the charge-density-wave and the Néel antiferromagnet orders are represented by the matrices  $\sigma_0 \beta_3$  and  $\sigma \beta_3$ , respectively, where  $\sigma = (\sigma_1, \sigma_2, \sigma_3)$  and two-component Pauli matrices  $\{\beta_{\mu}\}$  operate

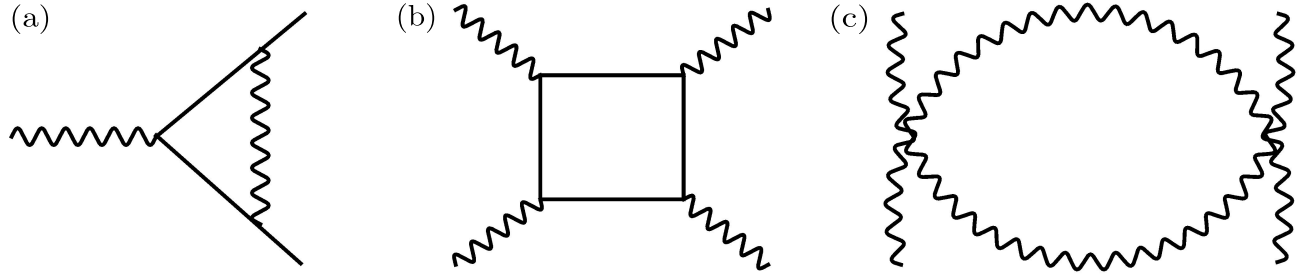

Figure S2. Leading-order correction for (a) the Yukawa vertex [Eq. (S14)] and (b)  $\Phi^4$ -vertex due to the Yukawa coupling [see Eq. (S14)]. (c) Leading-order correction for  $\Phi^4$ -vertex due to bosonic interaction ( $\lambda$ ).

on the sublattice degrees of freedom. Both the orders correspond to mass, as  $\{\sigma_0\beta_3, \sigma_0 h_0^{\text{lat}}(\mathbf{k})\} = \{\sigma\beta_3, \sigma_0 h_0^{\text{lat}}(\mathbf{k})\} = 0$ .

When we choose the mass matrix  $M = \sigma_0\beta_3$  in the NH Dirac operator  $H_{\text{NH}}$  [see Eq. (S1)], the anti-Hermitian operator  $M\sigma_0 h_0^{\text{lat}}(\mathbf{k})$  corresponds to nearest-neighbor hopping processes. But, the hopping amplitude in the direction of  $A$  to  $B$  sites is different from the one along the opposite direction, thus yielding non-Hermiticity. The Néel antiferromagnet order then becomes a CCM order, as now  $[M, \sigma\beta_3] = 0$ . Thus onsite Hubbard repulsion should favor nucleation of this order in such a NH Dirac system at weaker interactions in comparison to its counterpart in Hermitian graphene, as suggested by our mean-field susceptibility calculation. If, on the other hand, we choose  $M = \sigma_3\beta_3$ , the easy  $z$ -axis component of the Néel antiferromagnet, then this component corresponds to a CCM order. By contrast, the easy-plane XY component of the Néel antiferromagnet order represented by  $\sigma_{\perp}\beta_3$  becomes ACM order, where  $\sigma_{\perp} = (\sigma_1, \sigma_2)$ , as now  $\{\sigma_{\perp}\beta_3, M\} = 0$ . Then our susceptibility calculation suggests that on-site Hubbard repulsion should favor the nucleation of only the easy  $z$  axis Néel antiferromagnet order.

Identical conclusions hold in the continuum limit of  $h_0^{\text{lat}}(\mathbf{k})$ , featuring massless Dirac fermions around two inequivalent corners of the hexagonal Brillouin zone at  $\pm\mathbf{K}$  (also known as the valleys), where  $\mathbf{K} = (1/2, 1/(2\sqrt{3}))4\pi/(\sqrt{3}a)$ . Around these points, the linearized Dirac Hamiltonian for spinful fermions reads as

$$h_0 = v_{\text{H}} [\gamma_{031}k_x + \gamma_{002}k_y] \equiv v_{\text{H}} [\Gamma_1 k_x + \Gamma_2 k_y], \quad (\text{S38})$$

where  $v_{\text{H}} = \sqrt{3}t_0 a/2$ , the momentum  $\mathbf{k}$  is now measured from the respective valleys, and  $\gamma_{\mu\nu\rho} = \sigma_{\mu}\tau_{\nu}\beta_{\rho}$ . The newly introduced set of Pauli matrices  $\{\tau_{\mu}\}$  operate on the valley degrees of freedom. In this notation, the charge-density-wave and Néel antiferromagnet are represented by Hermitian mass matrices  $\gamma_{003}$  and  $\gamma_{j03}$ , respectively, where  $j = 1, 2, 3$ . Then all the discussions from the previous paragraph directly apply here as well.

## S6. GROSS-NEVEU-YUKAWA QUANTUM-CRITICAL THEORY

We here show the technical details leading to Eqs. (14), (15) and (17) in the main text, taking the GNY theory in the NH Yukawa-Lorentz symmetric hyperplane, i.e., when the effective Fermi velocity is equal to the bosonic one,  $v_{\text{F}} = v_{\text{B}}$ , with all three velocity components  $v_{\text{H}}$ ,  $v_{\text{NH}}$  and  $v_{\text{B}}$  being nonzero, as is the case for the CCM order parameter for which the mass matrices satisfy  $\{N_j, N_k\} = 2\delta_{jk}$  and  $[N_j, M] = 0$  for  $j, k = 1, \dots, n$ . In particular, we show the details of the calculations of the Yukawa vertex [Fig. S2(a)] and the  $\Phi^4$ -vertex [Fig. S2(b)] corrections arising from the fermions.

The form of the Yukawa vertex correction [Fig. S2(a)] is given by

$$\delta g = g^3 \frac{1}{4N_f} \sum_{k=1}^n \text{Tr} \left[ N_j \int_{\omega, \mathbf{k}} N_k G_{\text{F}} N_j G_{\text{F}} N_k G_{\text{B}} \right], \quad (\text{S39})$$

where  $\int_{\omega, \mathbf{k}} \equiv \int \frac{d\omega}{2\pi} \frac{d^d \mathbf{k}}{(2\pi)^d}$ , while  $G_{\text{F}} \equiv G_{\text{F}}(i\omega, \mathbf{k})$  and  $G_{\text{B}} \equiv G_{\text{B}}(i\omega, \mathbf{k})$ , are the fermionic and bosonic propagators given in Eq. (S3) and (S16), respectively. After setting  $v_{\text{F}} = v_{\text{B}}$  (critical NH Yukawa-Lorentz symmetric hyperplane), we

find

$$\delta g = (n-2)g^3 \int_{\omega, \mathbf{k}} \frac{1}{(\omega^2 + v_F^2 k^2)^2} = (n-2)g^3 \left( \frac{1}{8\pi^2} \right) \left( \frac{1}{4v_F^3} \right) \left( \frac{1}{\varepsilon} \right), \quad (\text{S40})$$

where in the last step we set  $d = 3 - \varepsilon$ . Contribution of this diagram is identical for the ACM order parameter for which  $\{N_j, N_k\} = 2\delta_{jk}$  and  $\{N_j, M\} = 0$  for  $j, k = 1, \dots, n$ , except  $v_F \rightarrow v_H$  since on the corresponding Yukawa-Lorentz symmetric hyperplane  $v_{NH} = 0$  and  $v_H = v_B$ .

The correction of the  $\Phi^4$  vertex arising from the Yukawa interaction [Fig. S2(b)] reads as

$$\delta \lambda_g = g^4 \text{Tr} \left[ \int_{\omega, \mathbf{k}} G_F N G_F N G_F N G_F N \right], \quad (\text{S41})$$

which after using that the mass matrix  $N$  belongs to the CCM order parameter and taking the trace, reads

$$\delta \lambda_g = 4N_f \int_{\omega, \mathbf{k}} \frac{1}{(\omega^2 + v_F^2 k^2)^2} = N_f \frac{g^4}{8\pi^2 v_F^3 \varepsilon}. \quad (\text{S42})$$

Contribution of this diagram is identical for the ACM order parameter, except  $v_F \rightarrow v_H$ .

For the sake of completeness we briefly outline the  $\Phi^4$ -vertex correction due to the boson self-interaction ( $\lambda$ ). See Fig. S2(c). In terms of the bosonic velocity ( $v_B$ ) it is given by

$$\delta \lambda_\lambda = \lambda^2 \int_{\omega, \mathbf{k}} G_B G_B = \lambda^2 \left( \frac{1}{8\pi^2} \right) \left( \frac{1}{4v_B^3} \right) \left( \frac{1}{\varepsilon} \right). \quad (\text{S43})$$

Near the CCM ordering  $v_B = v_F$ , while near the ACM ordering  $v_B = v_H$ .

Using these results, together with the corresponding renormalization conditions for the Yukawa and the  $\Phi^4$  couplings, and the fermionic and bosonic field renormalizations given by Eq. (S20) and (S33), respectively, we find Eqs. (14), (15) and (17) of the main text.
